# Supplementary material for: A Comparison of Rendering Techniques for Large 3D Line Sets with Transparency
Source: arXiv:1912.08485 source file (2020-07-31)
Supplement: Supplementary file 3 [file appendix_performances.tex]

% \clearpage

\input{content/error_points_appendix}

\clearpage
\begin{figure*}[!hb]	
	\centering
	\begin{overpic}[width=0.245\textwidth,clip,trim= 0mm 10mm 2mm 2mm]
		{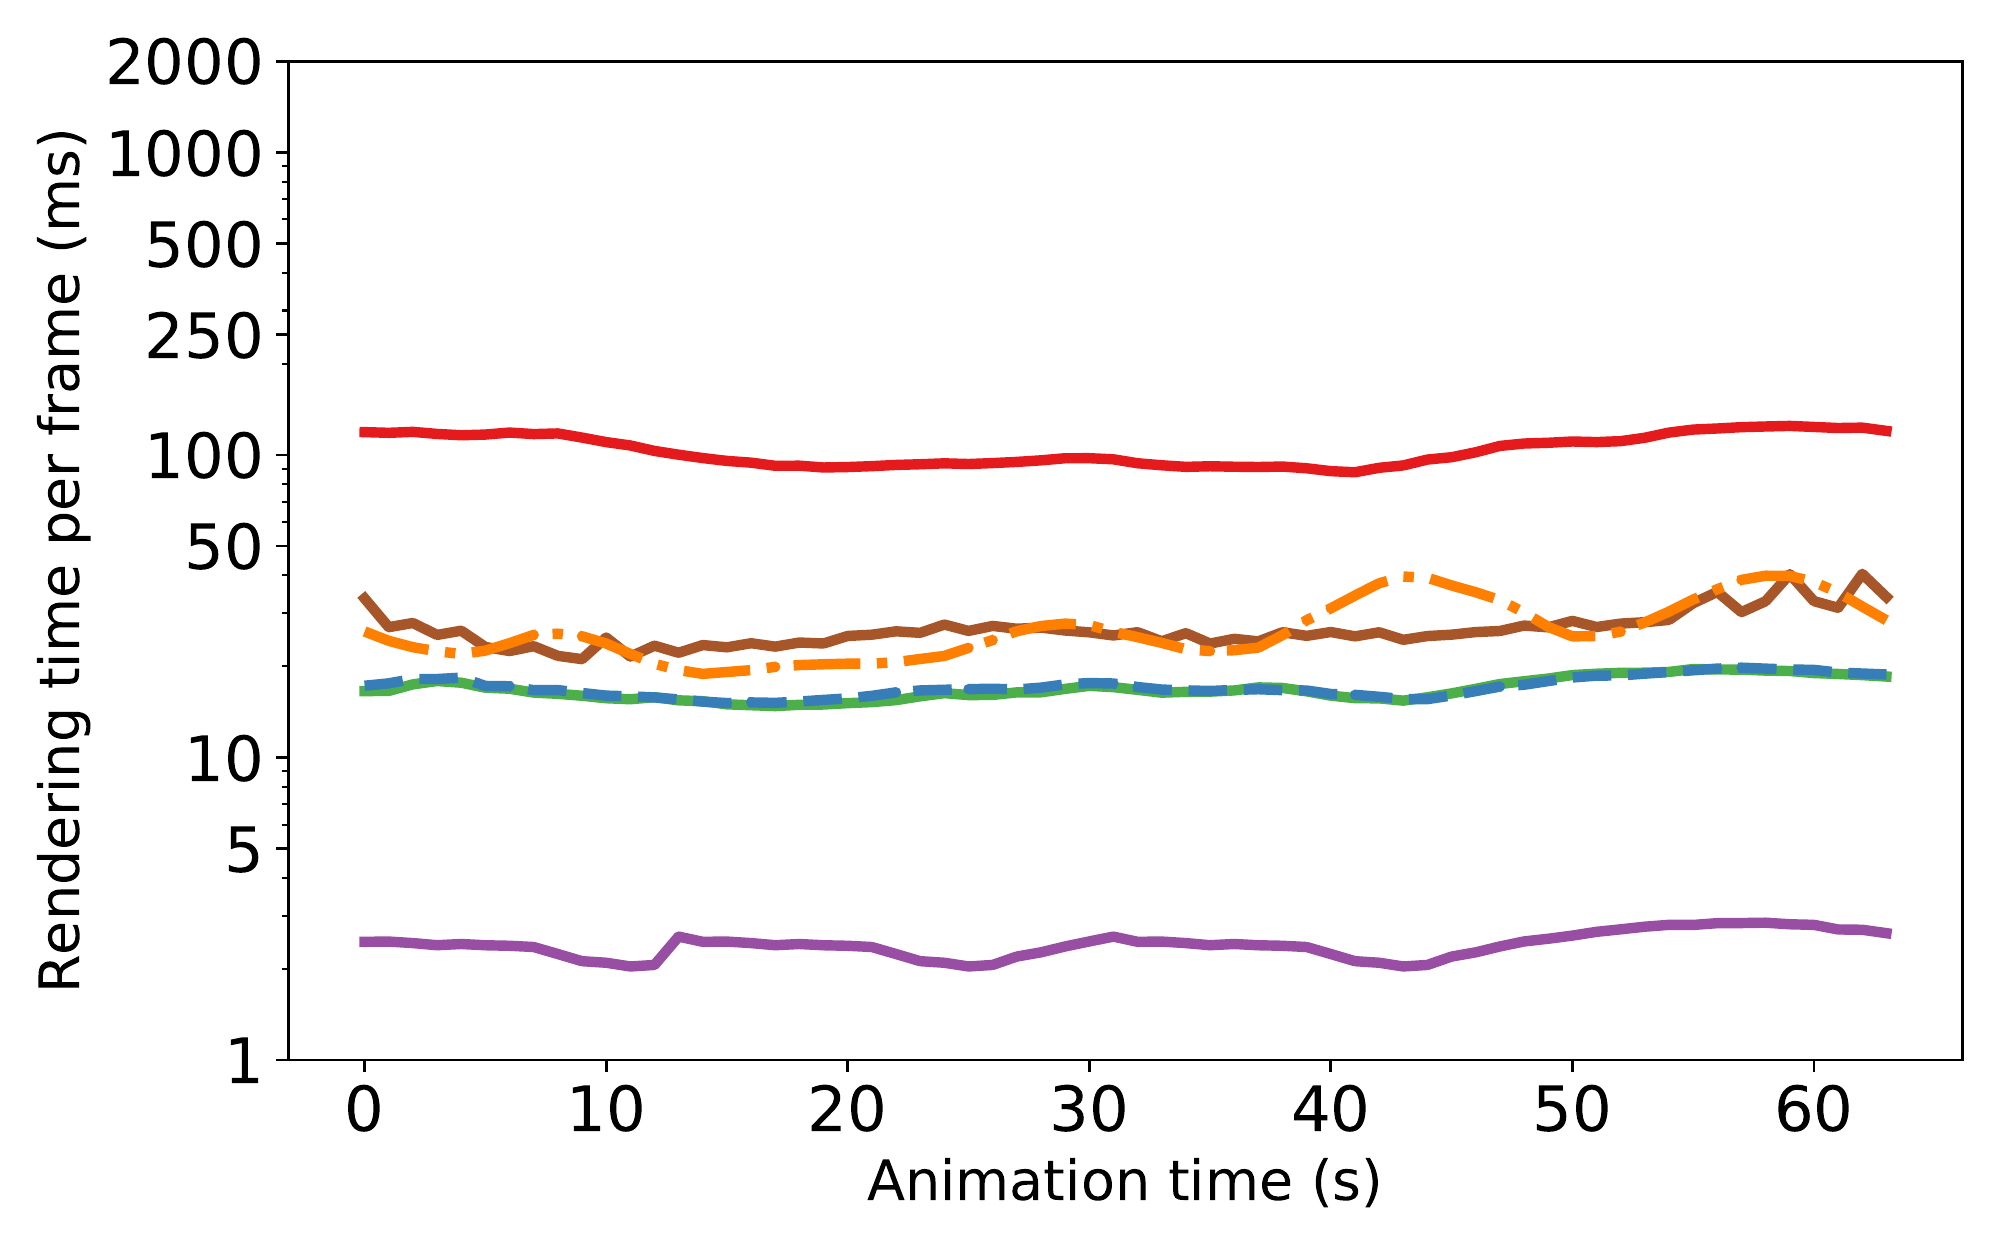}
	\end{overpic}%
	\begin{overpic}[width=0.245\textwidth,,clip,trim= 0mm 10mm 2mm 2mm]
		{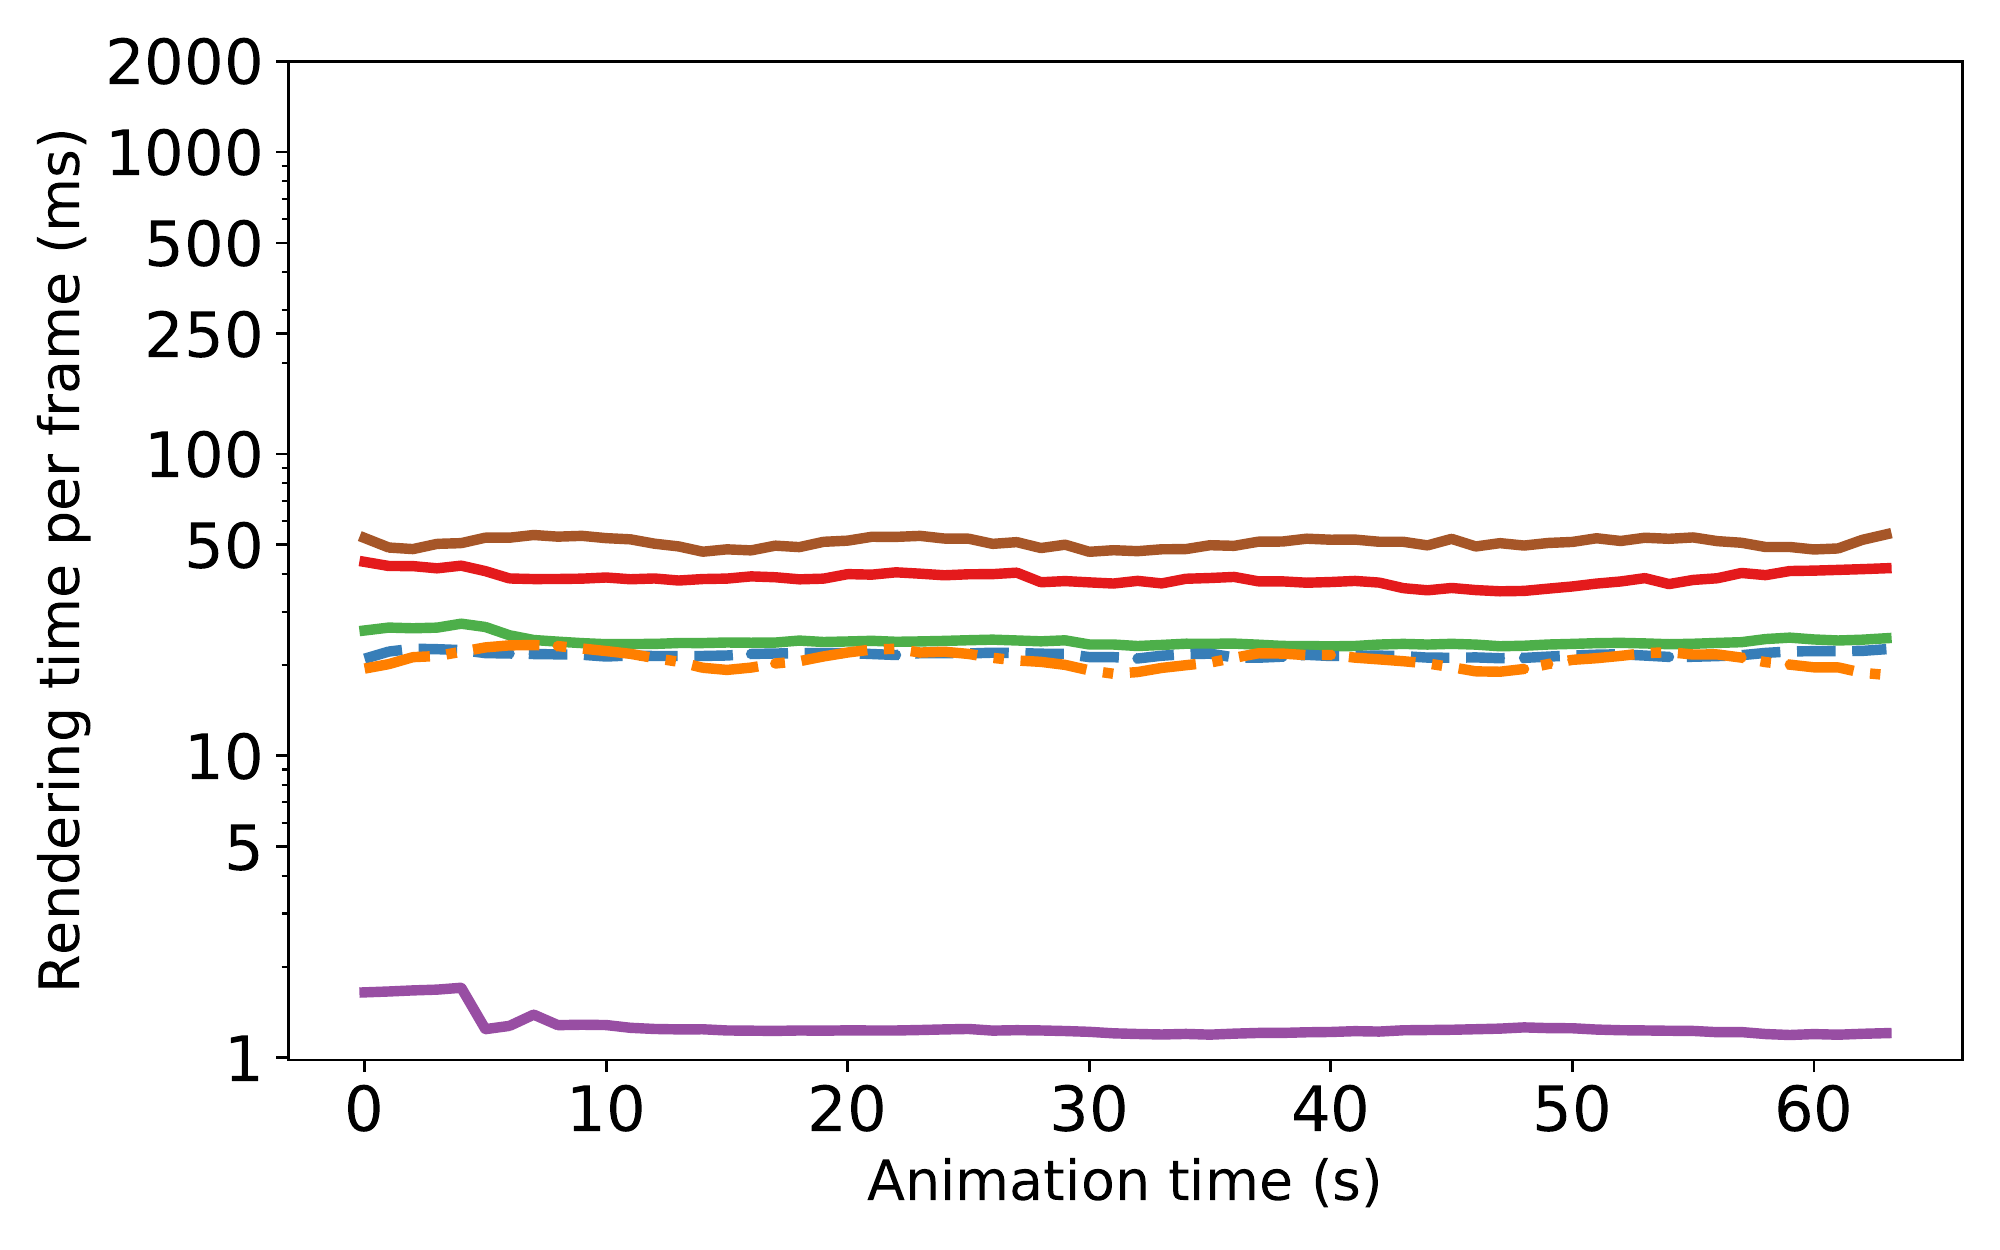}
	\end{overpic}%
	\begin{overpic}[width=0.245\textwidth,clip,trim= 0mm 10mm 2mm 2mm]
		{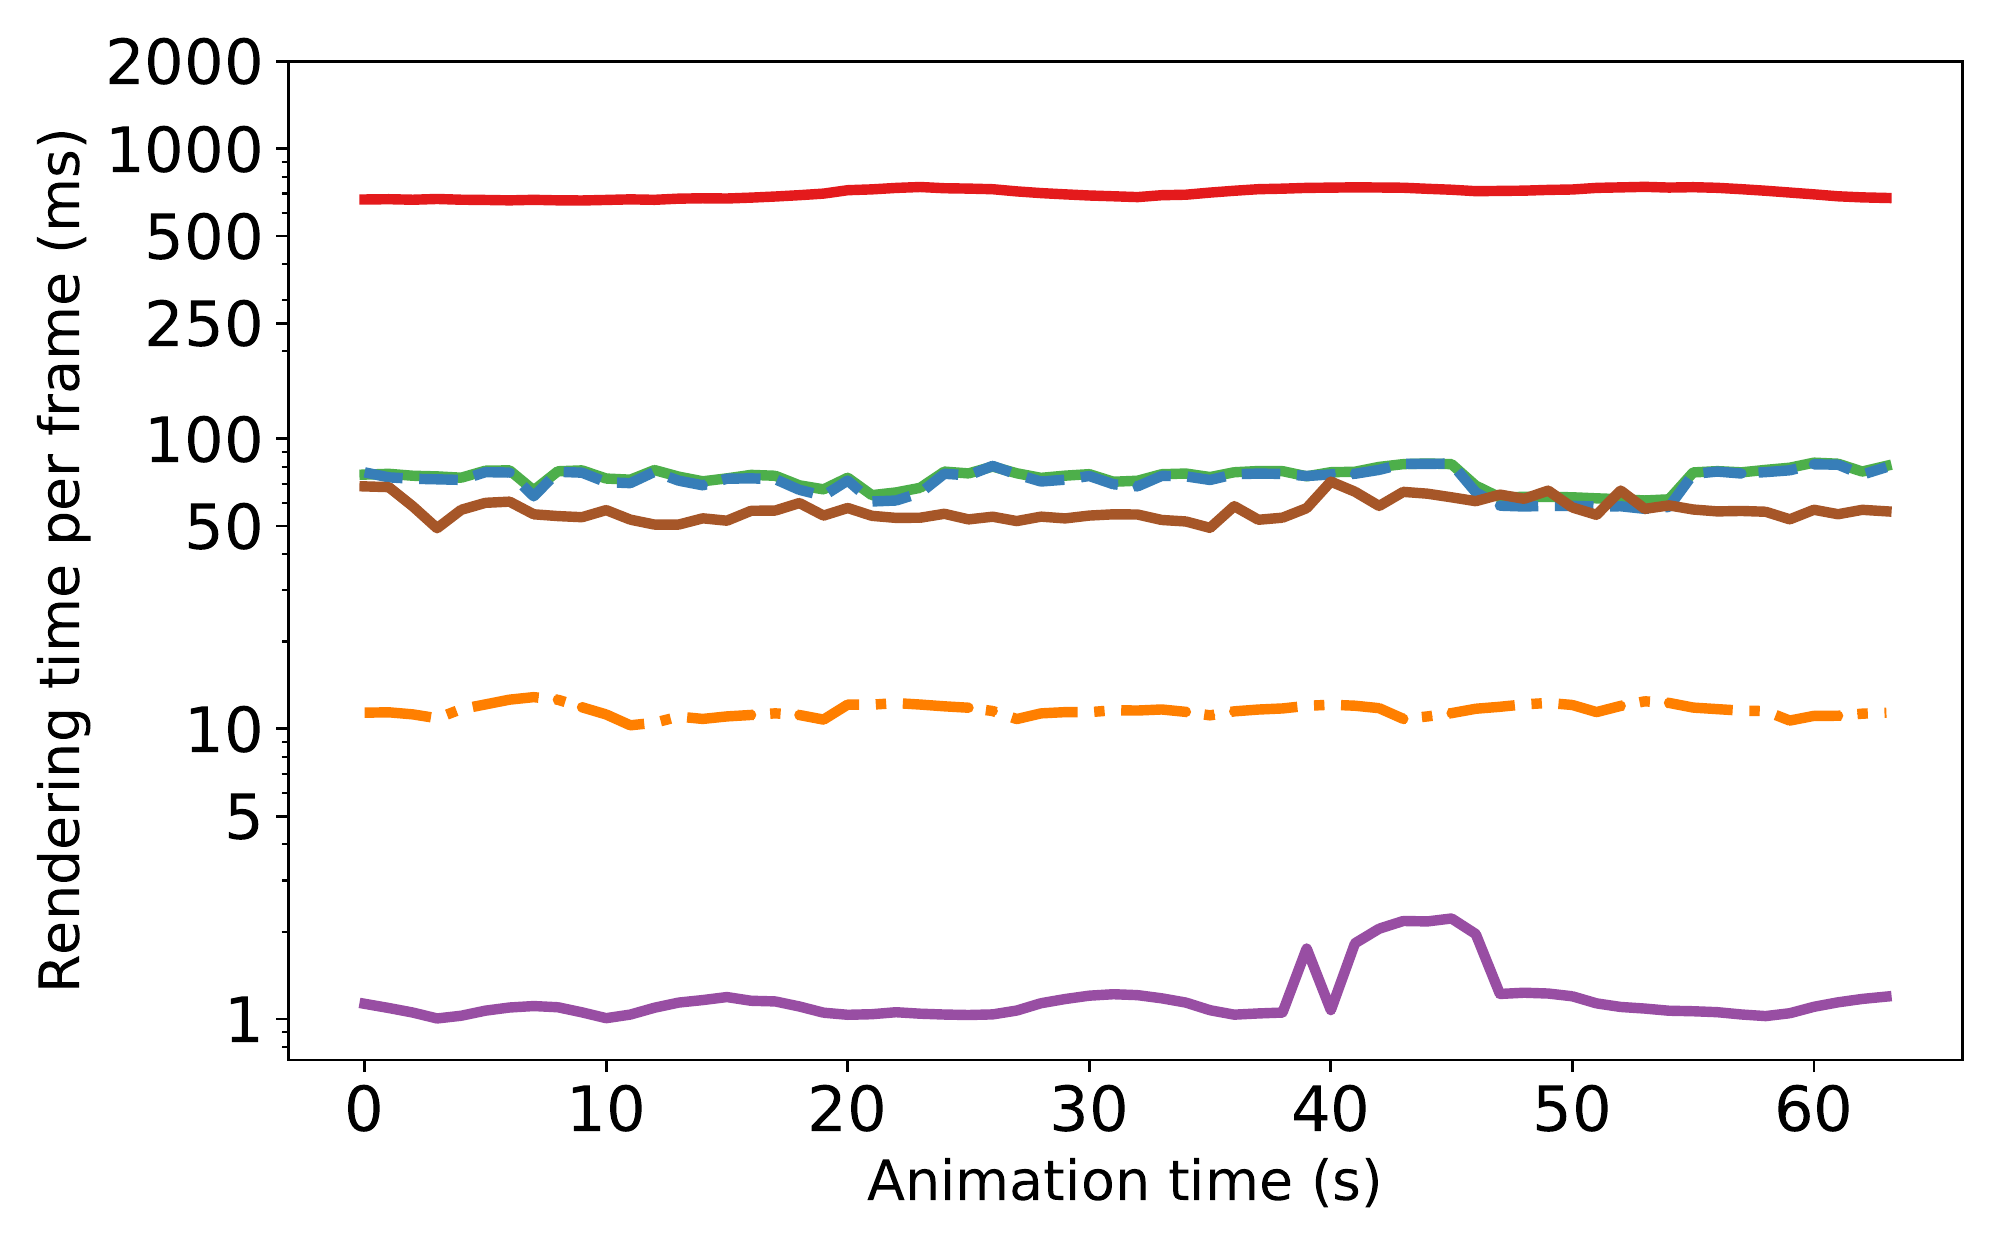}
	\end{overpic}%
	\begin{overpic}[width=0.245\textwidth,clip,trim= 0mm 10mm 2mm 2mm]
		{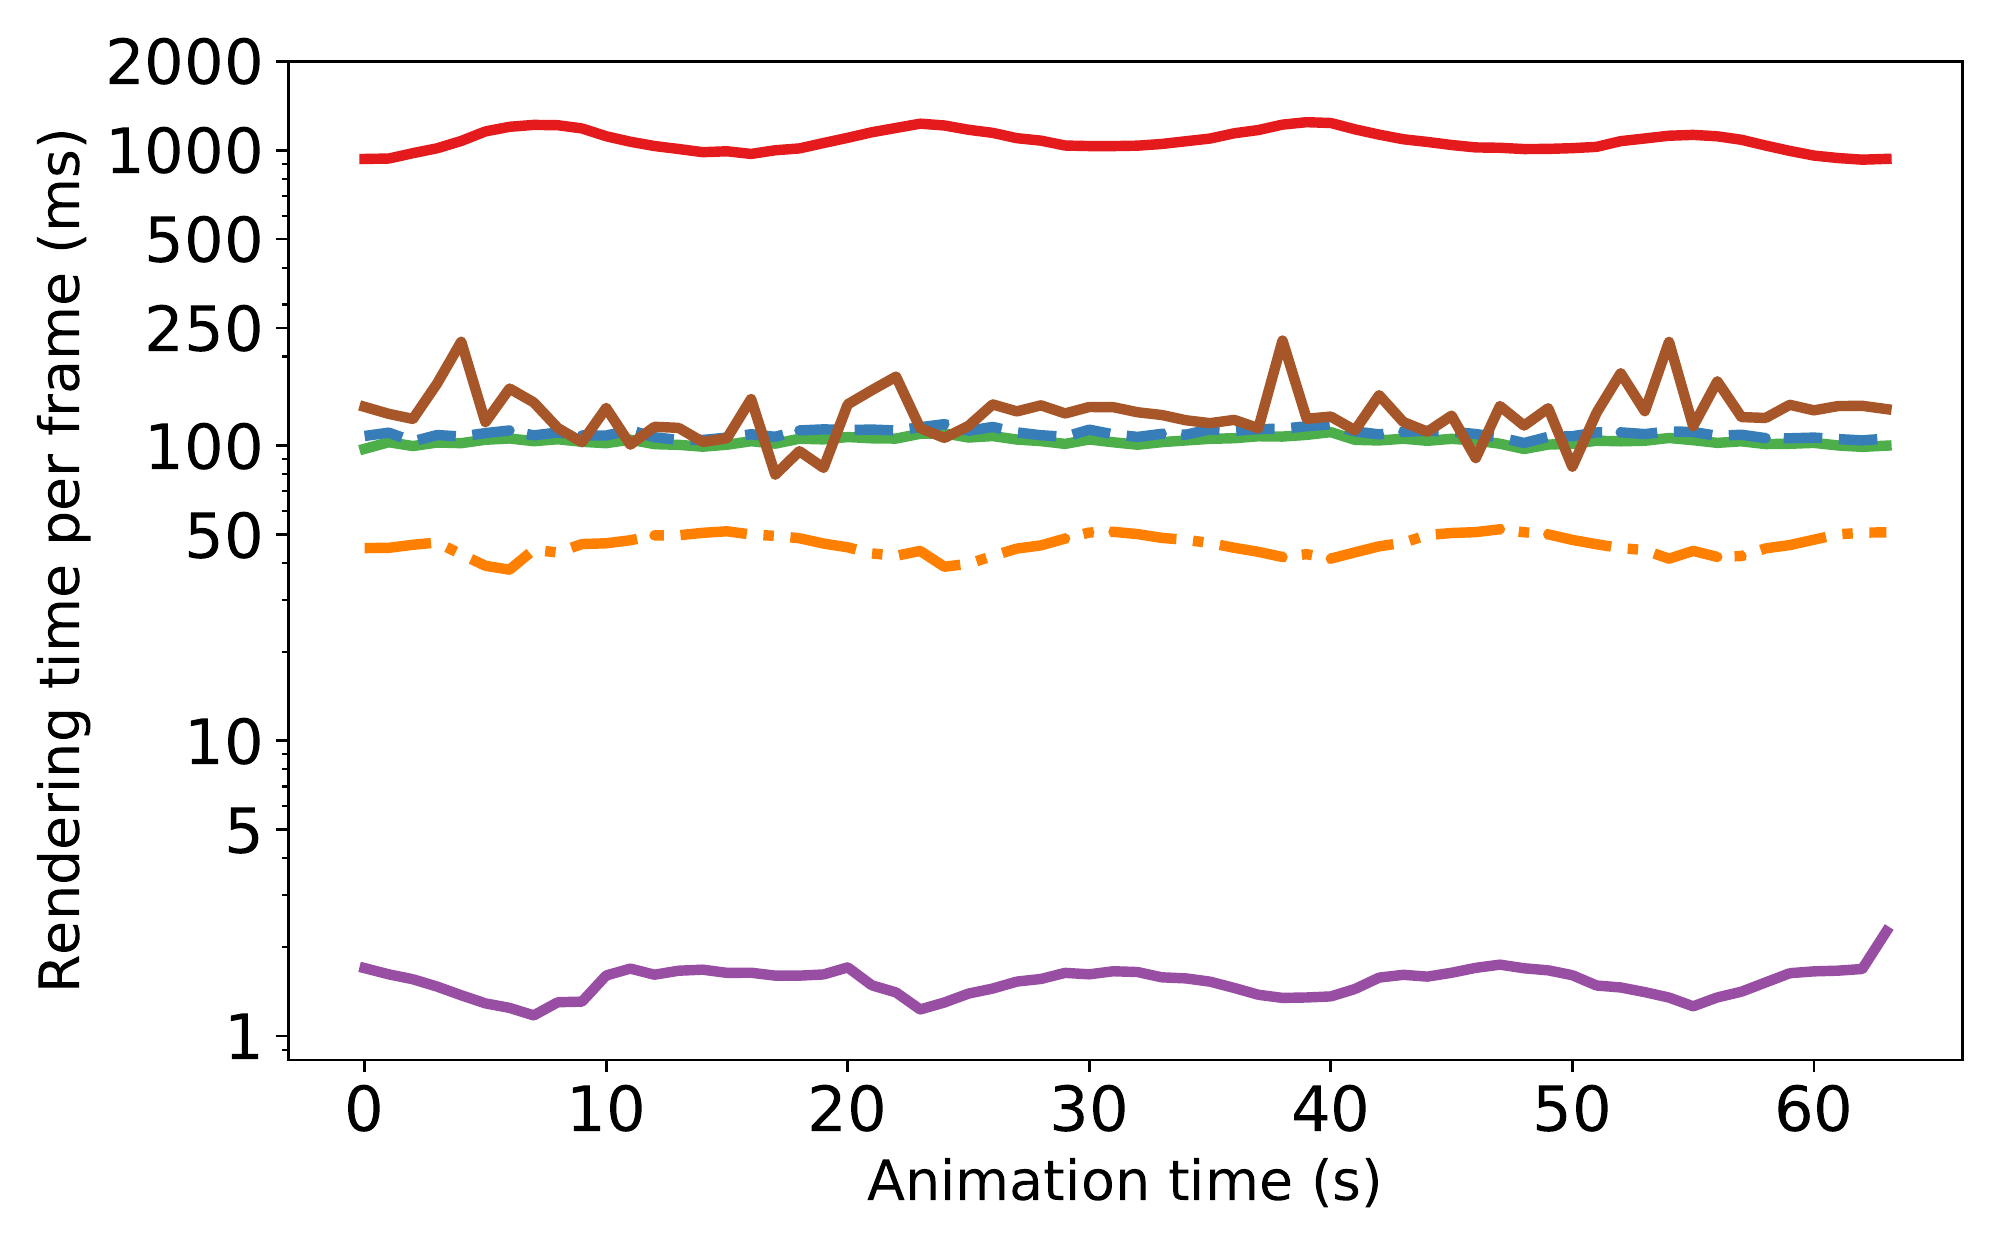}
	\end{overpic}

	\begin{overpic}[width=0.245\textwidth,clip,trim= 00mm 10mm 2mm 2mm]
		{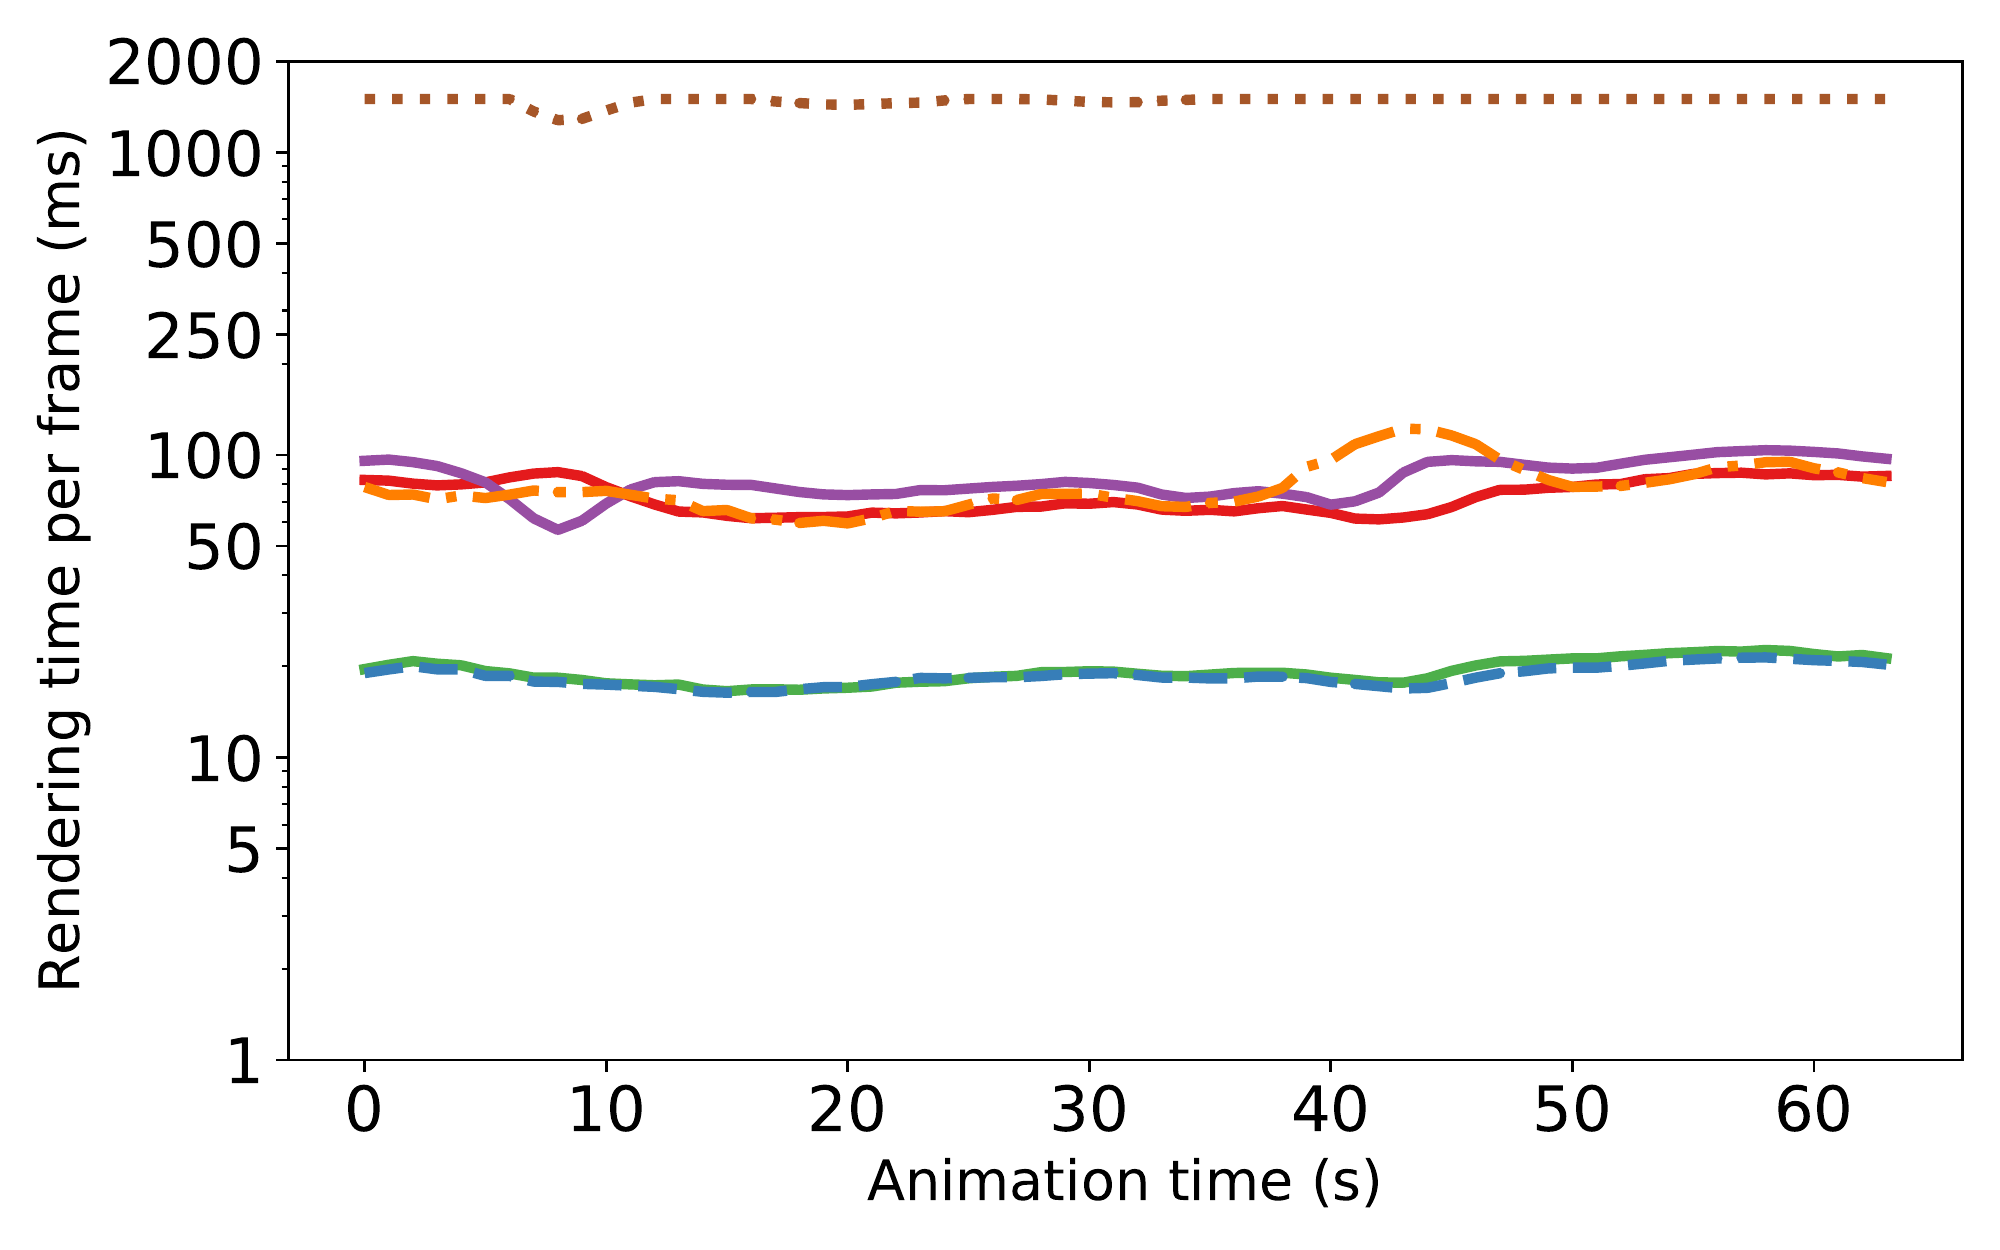}
	\end{overpic}%
	\begin{overpic}[width=0.245\textwidth,clip,trim= 00mm 10mm 2mm 2mm]
		{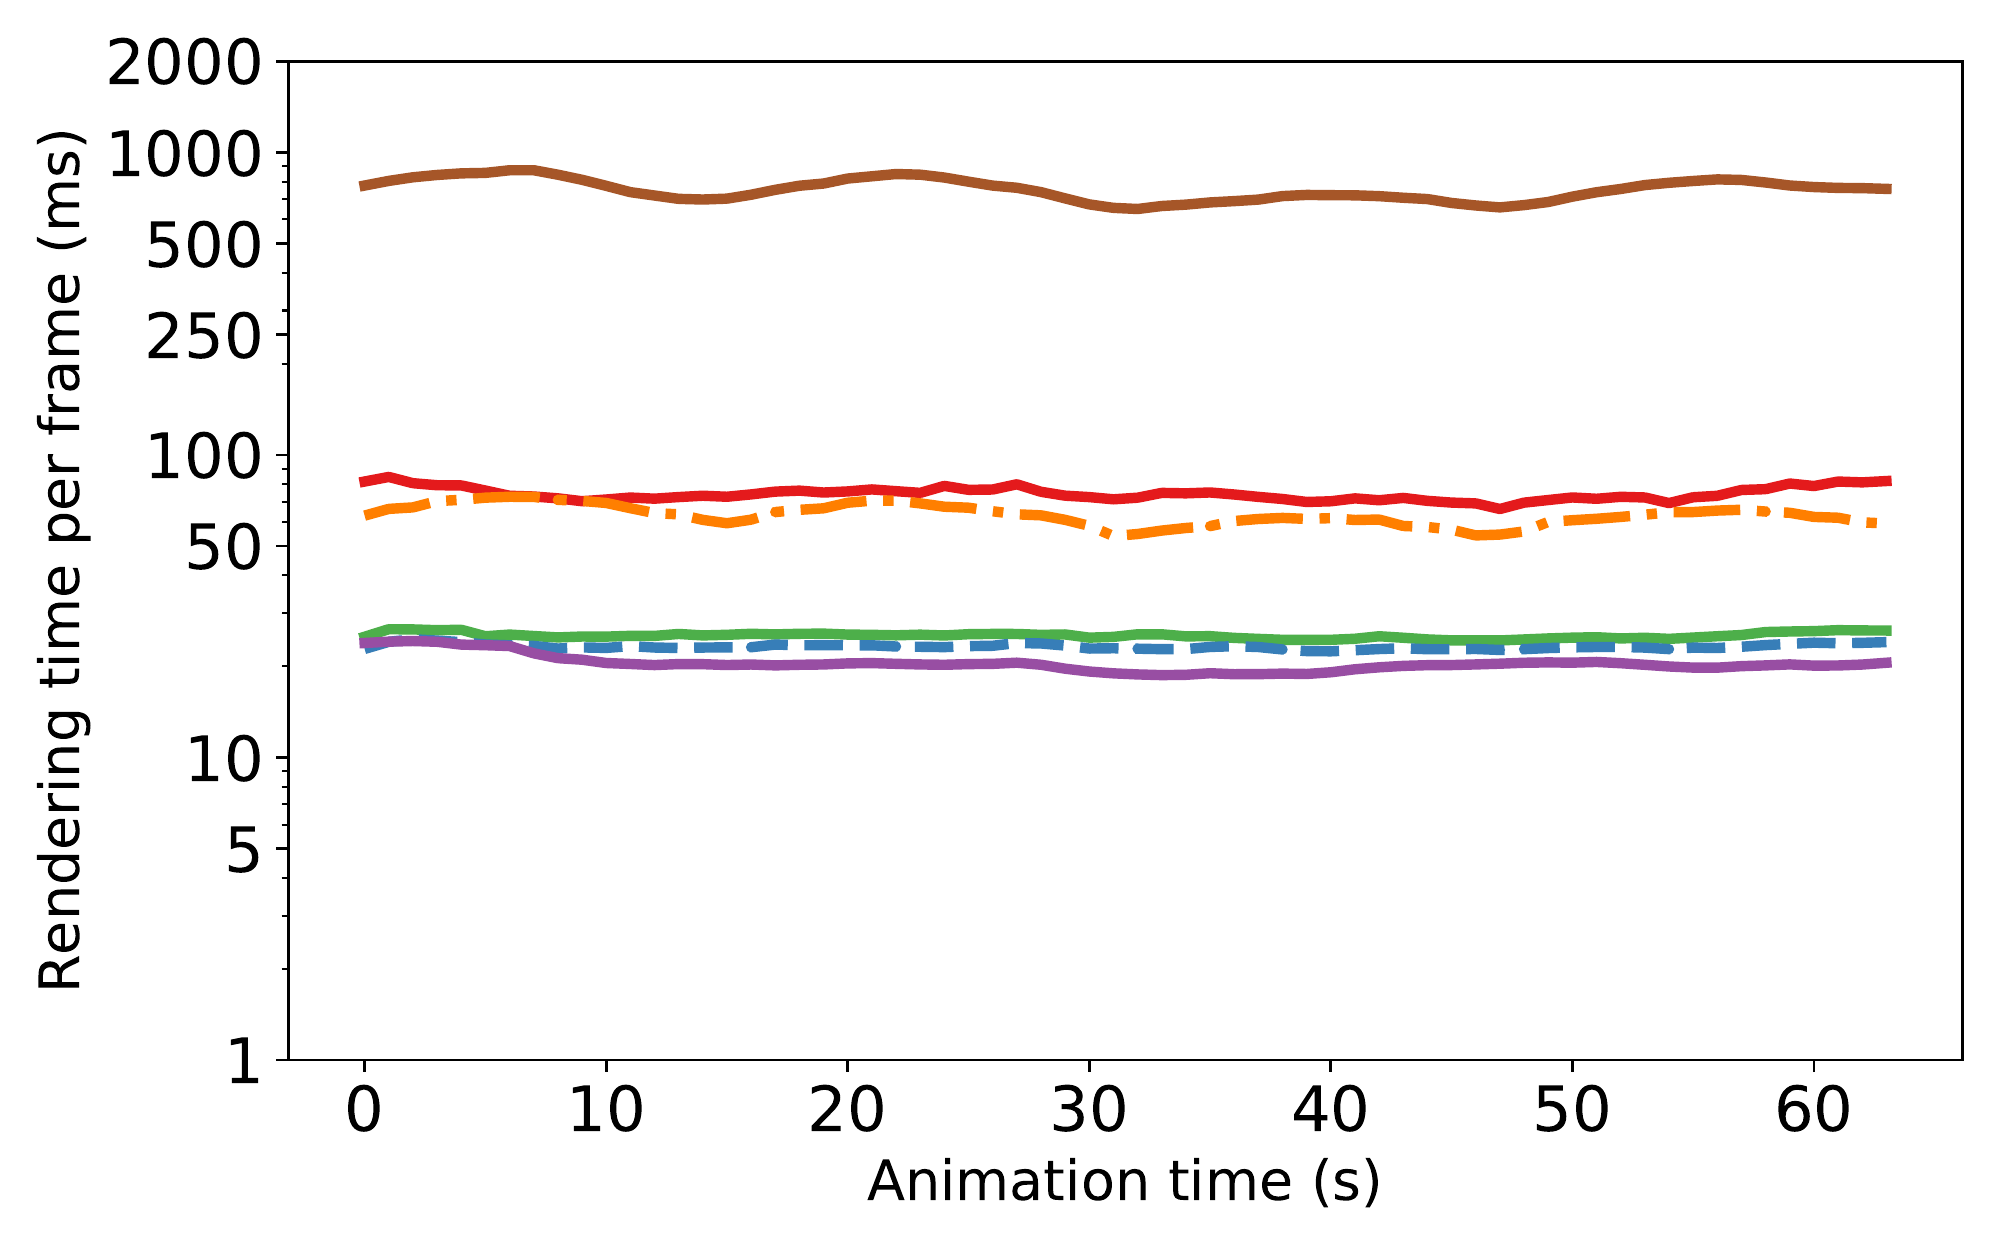}
	\end{overpic}%
	\begin{overpic}[width=0.245\textwidth,clip,trim= 00mm 10mm 2mm 2mm]
		{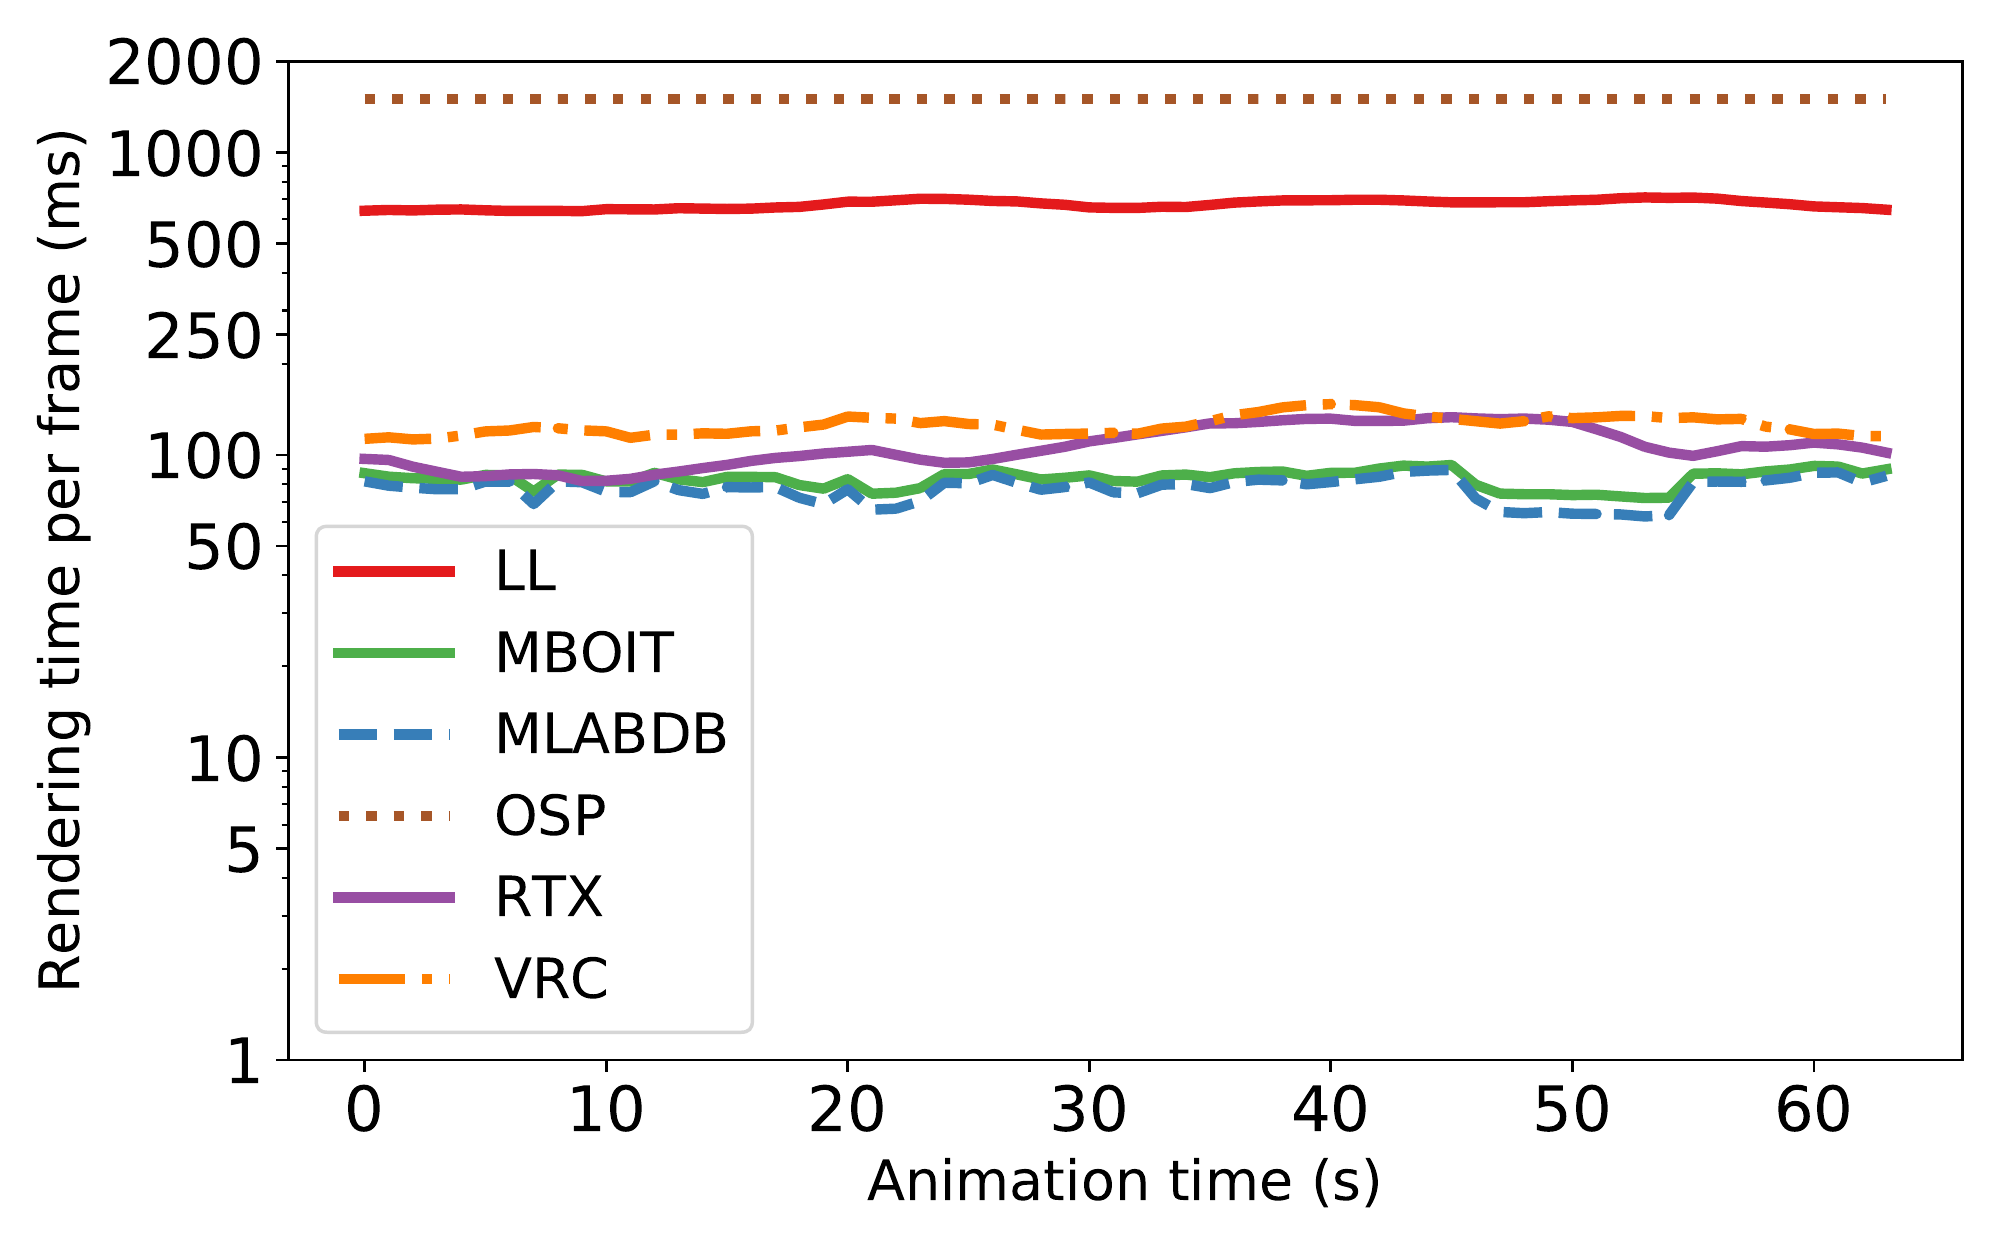}
	\end{overpic}%
	\begin{overpic}[width=0.245\textwidth,clip,trim= 00mm 10mm 2mm 2mm]
		{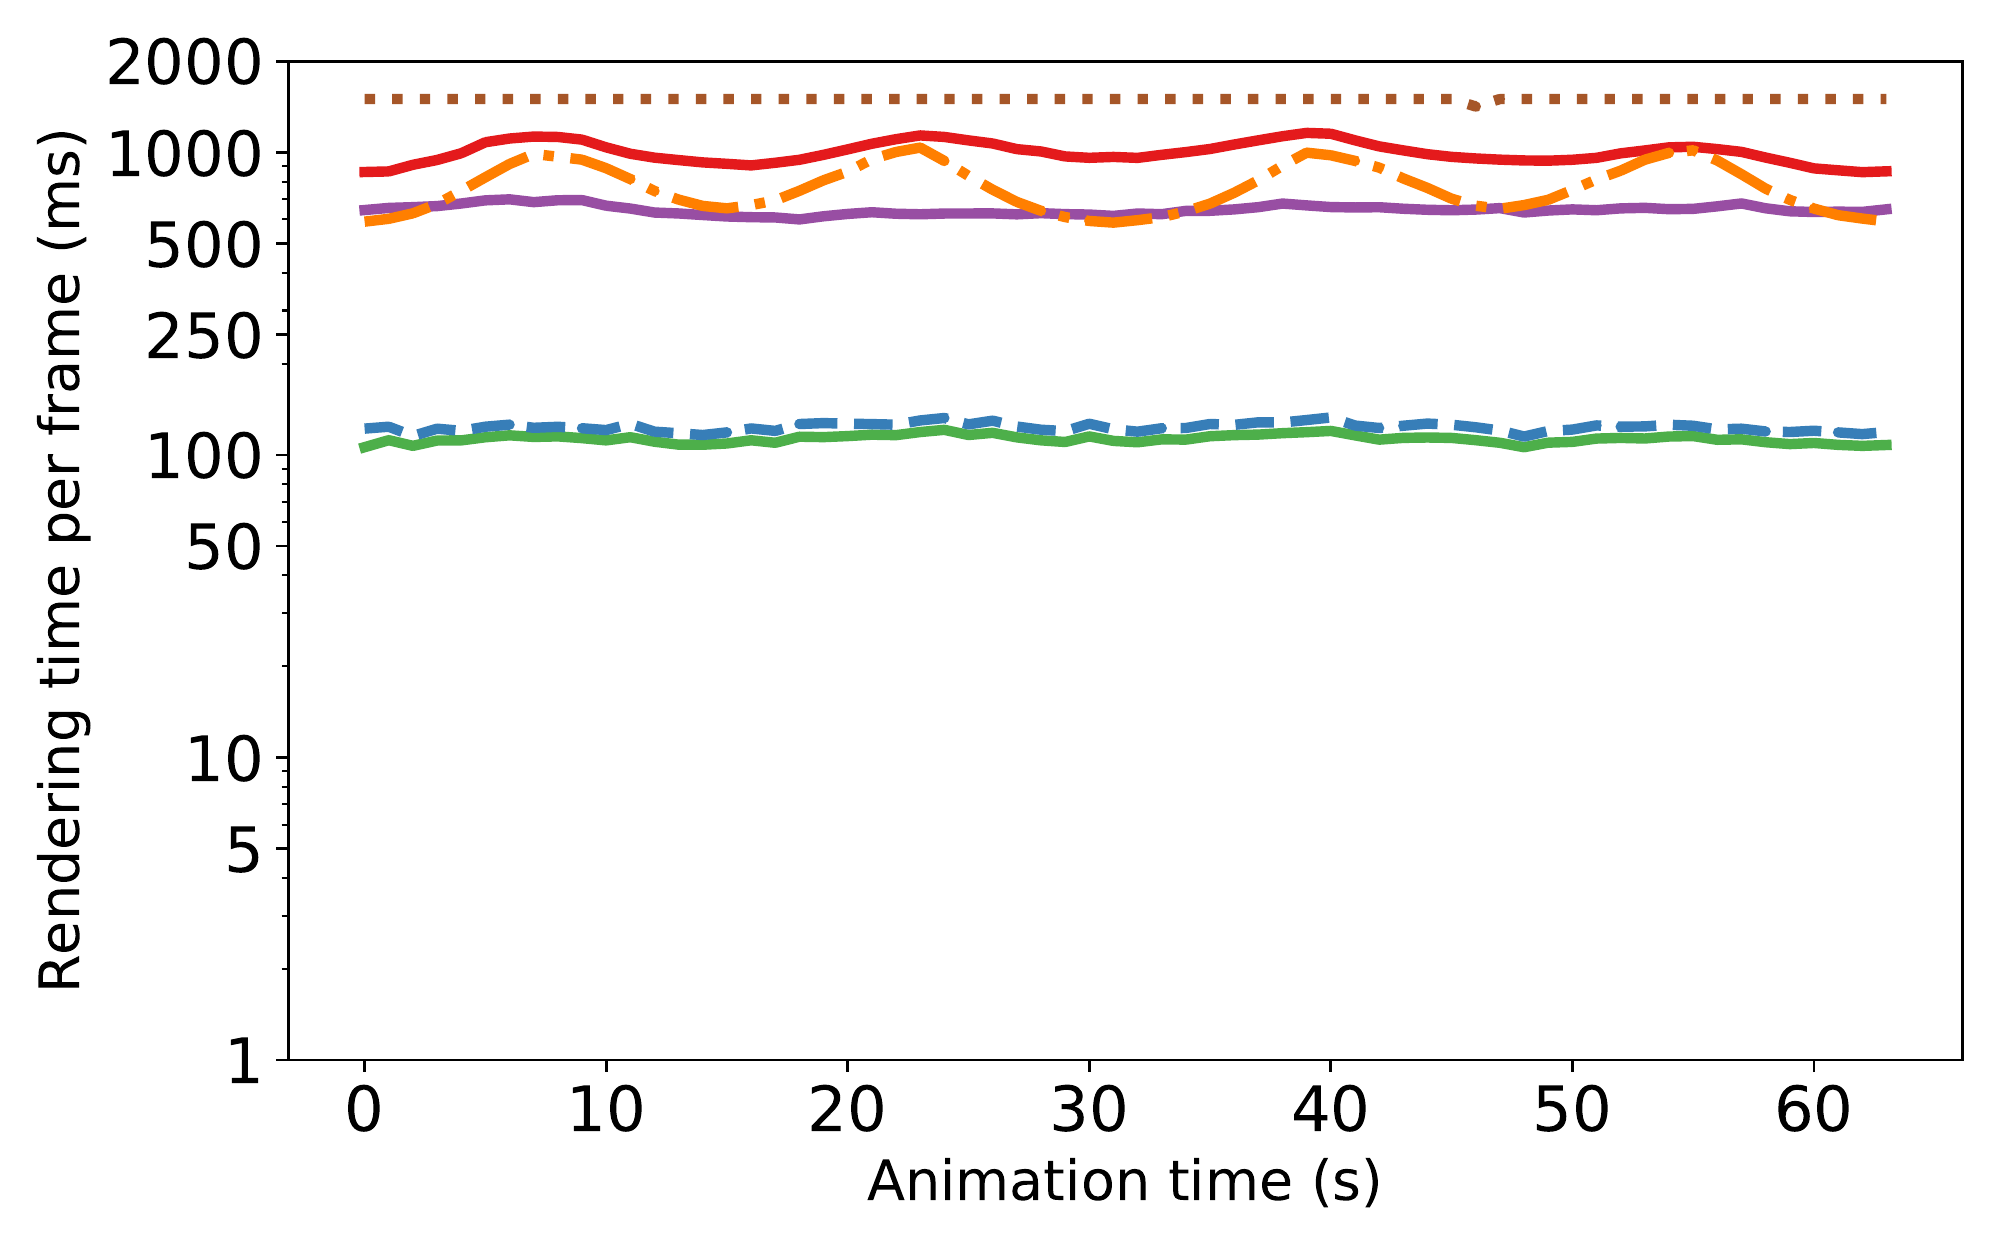}
	\end{overpic}

	\begin{overpic}[width=0.245\textwidth,clip,trim= 00mm 0mm 2mm 2mm]
		{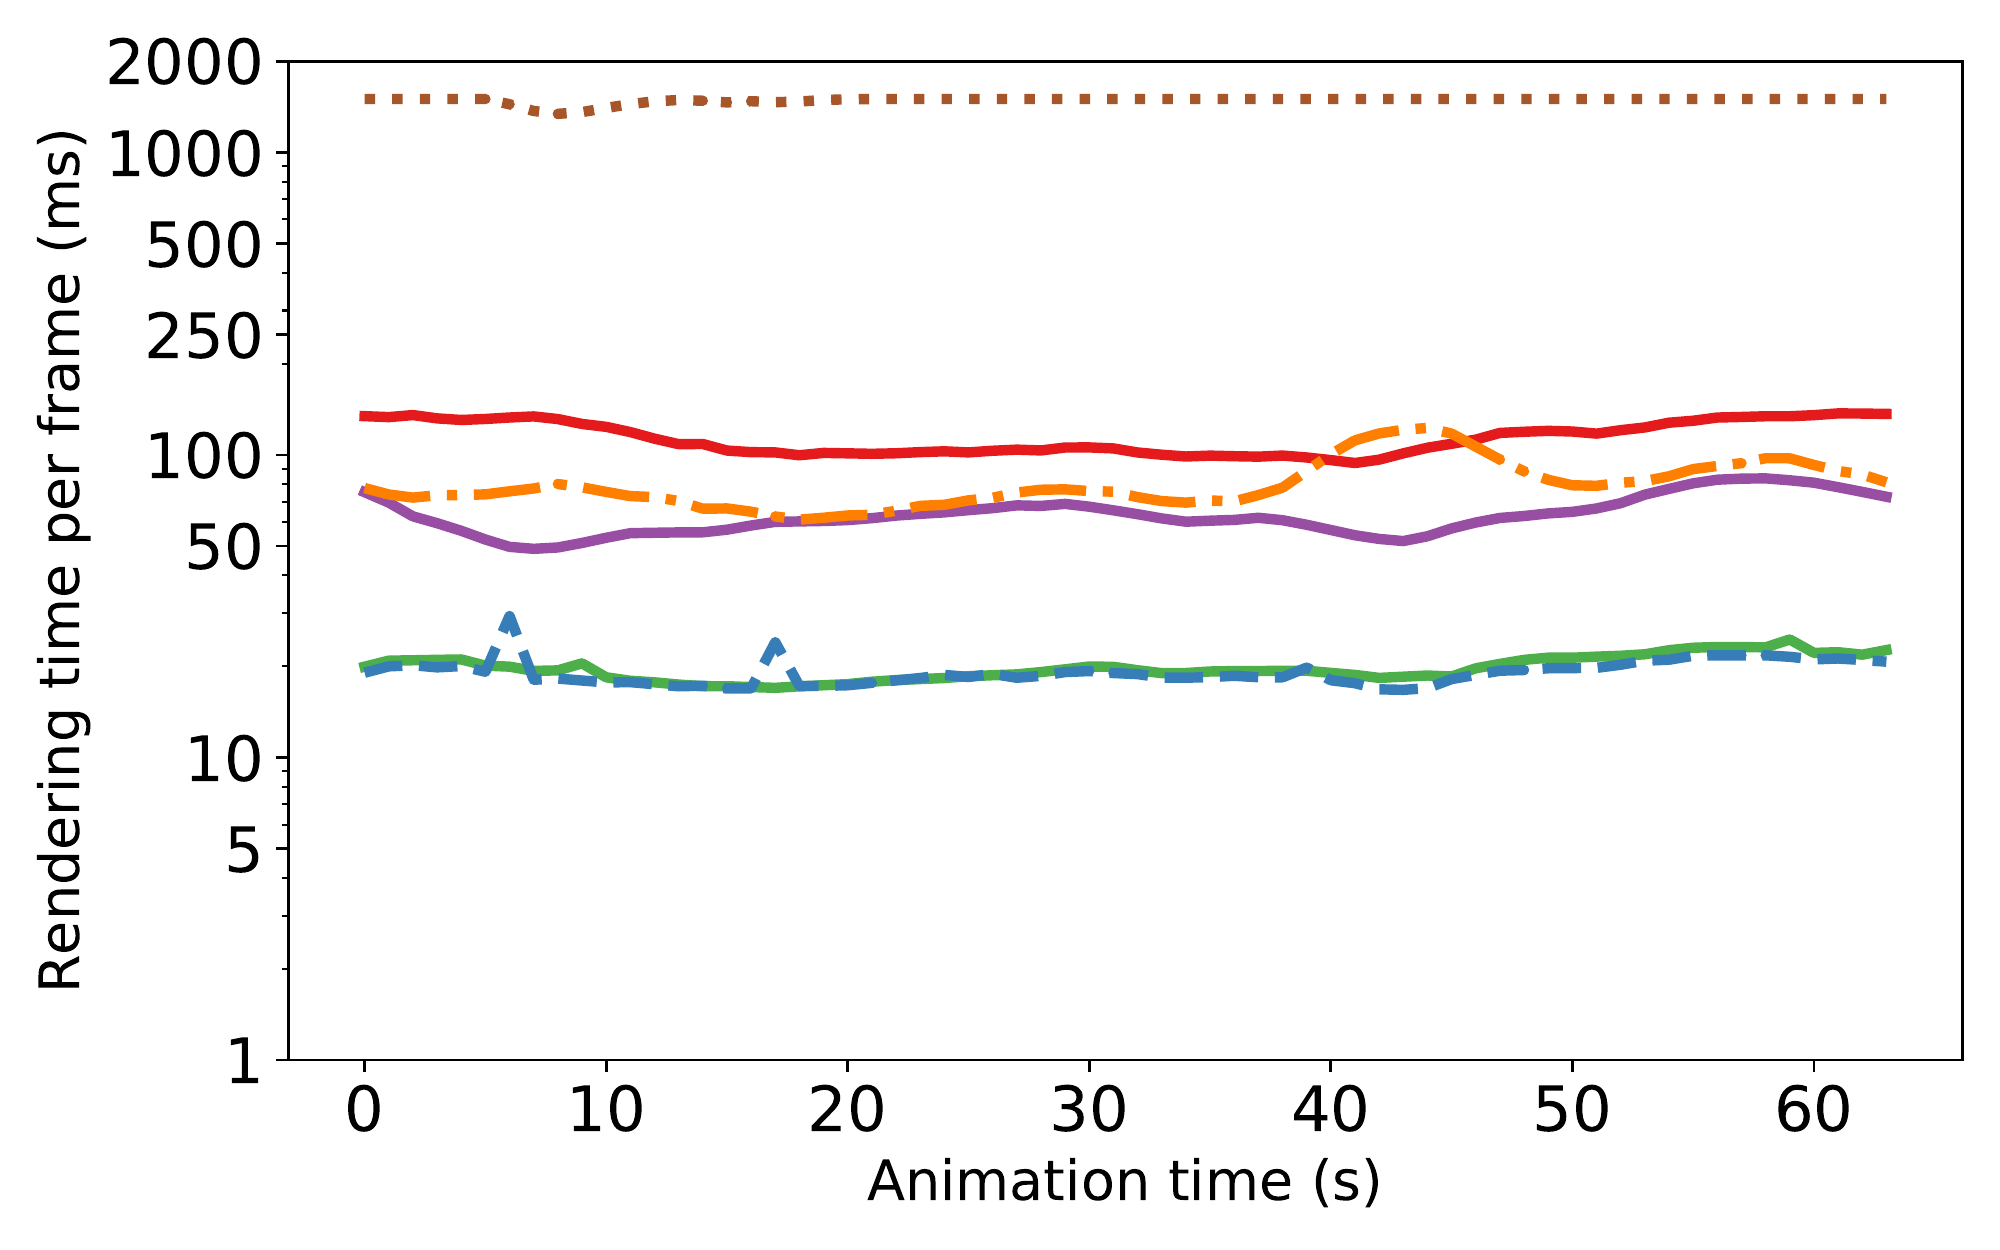}
		\put(38,15){\scriptsize\textbf{\textcolor{gray}{ANEURYSM}}}
	\end{overpic}%
	\begin{overpic}[width=0.245\textwidth,clip,trim= 00mm 0mm 2mm 2mm]
		{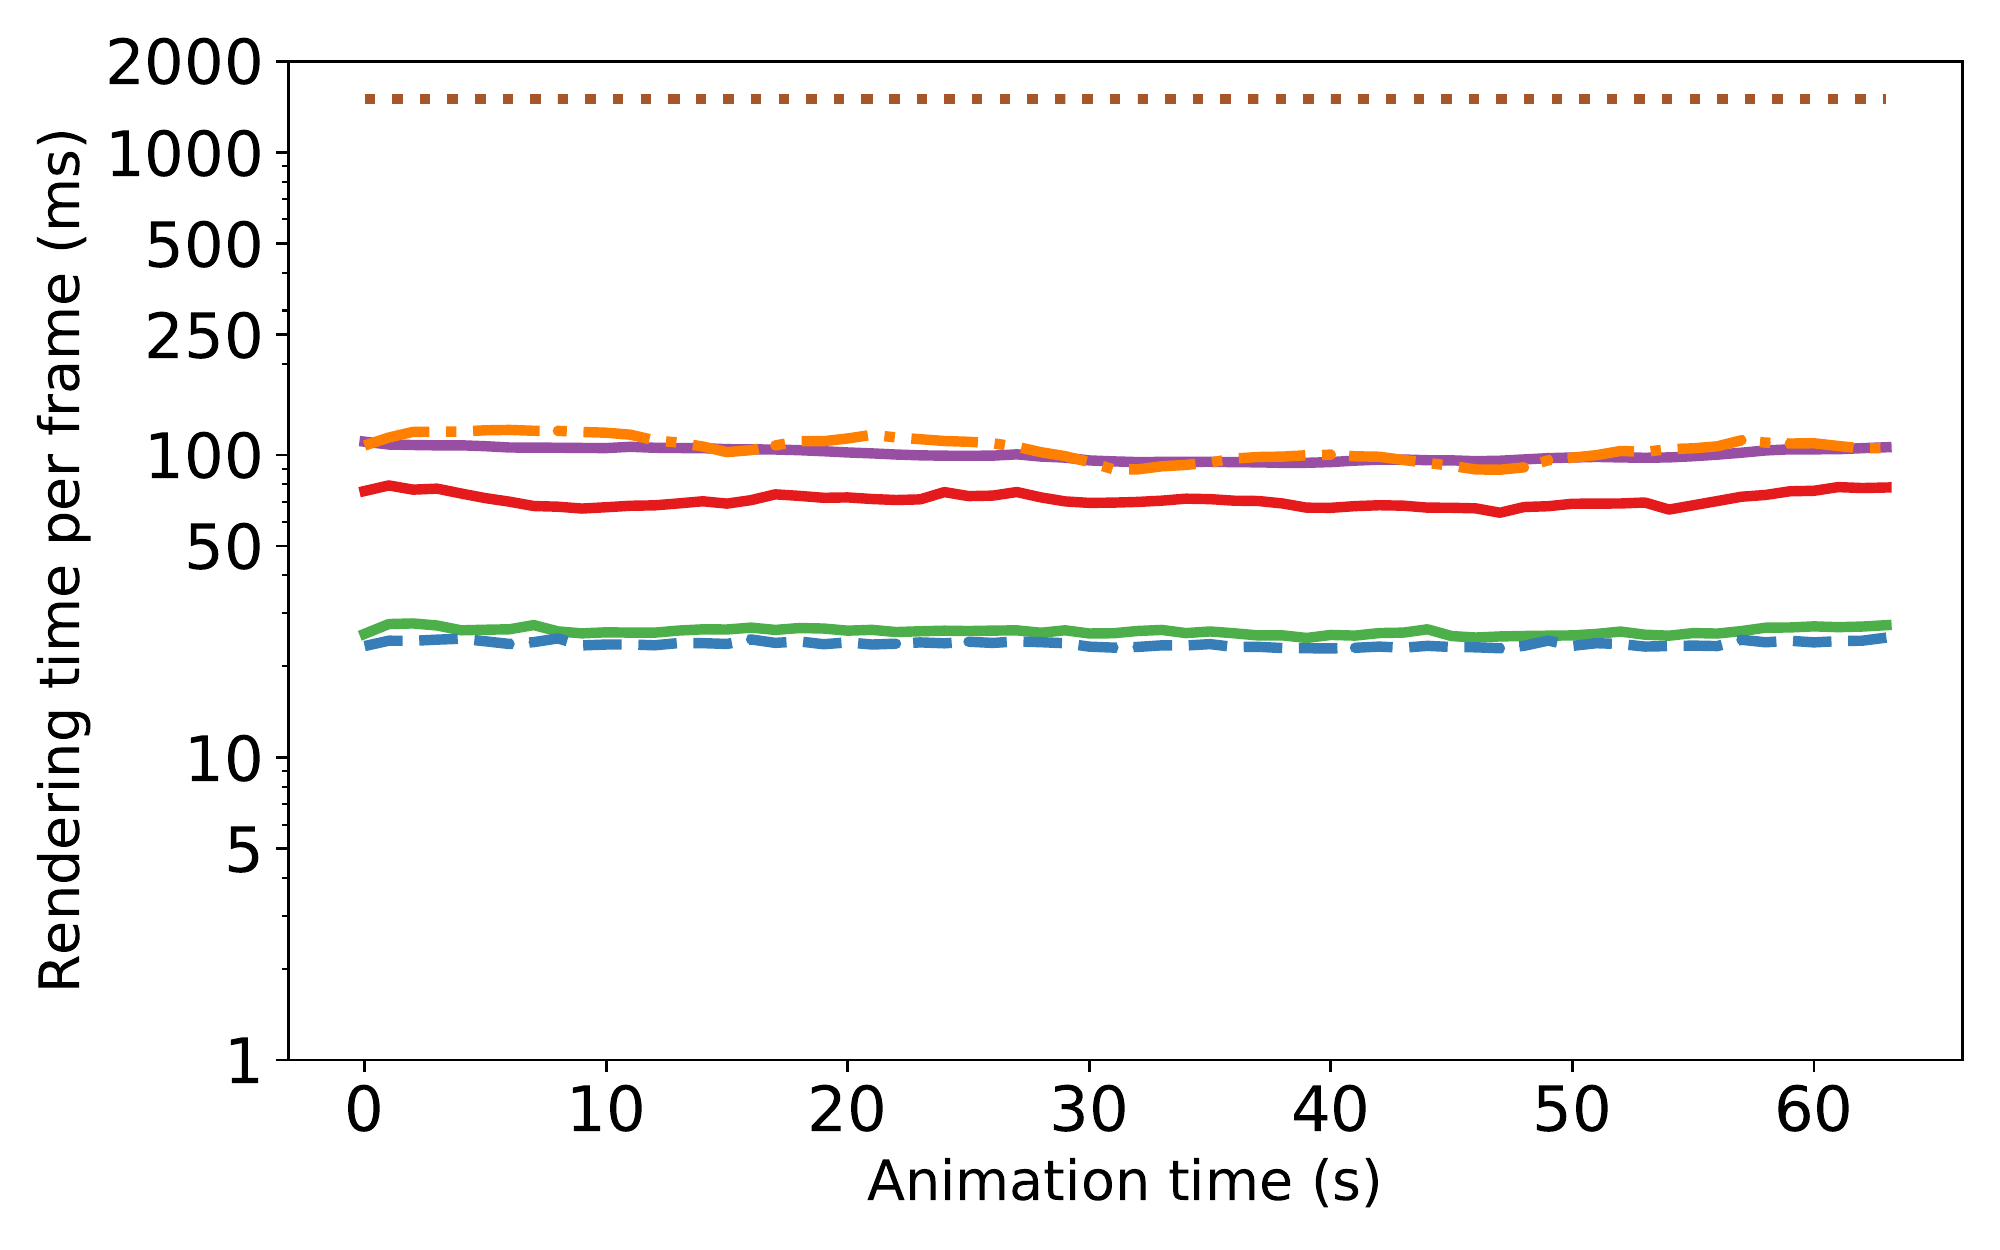}
		\put(34,15){\scriptsize\textbf{\textcolor{gray}{CONVECTION}}}
	\end{overpic}%
	\begin{overpic}[width=0.245\textwidth,clip,trim= 00mm 0mm 2mm 2mm]
		{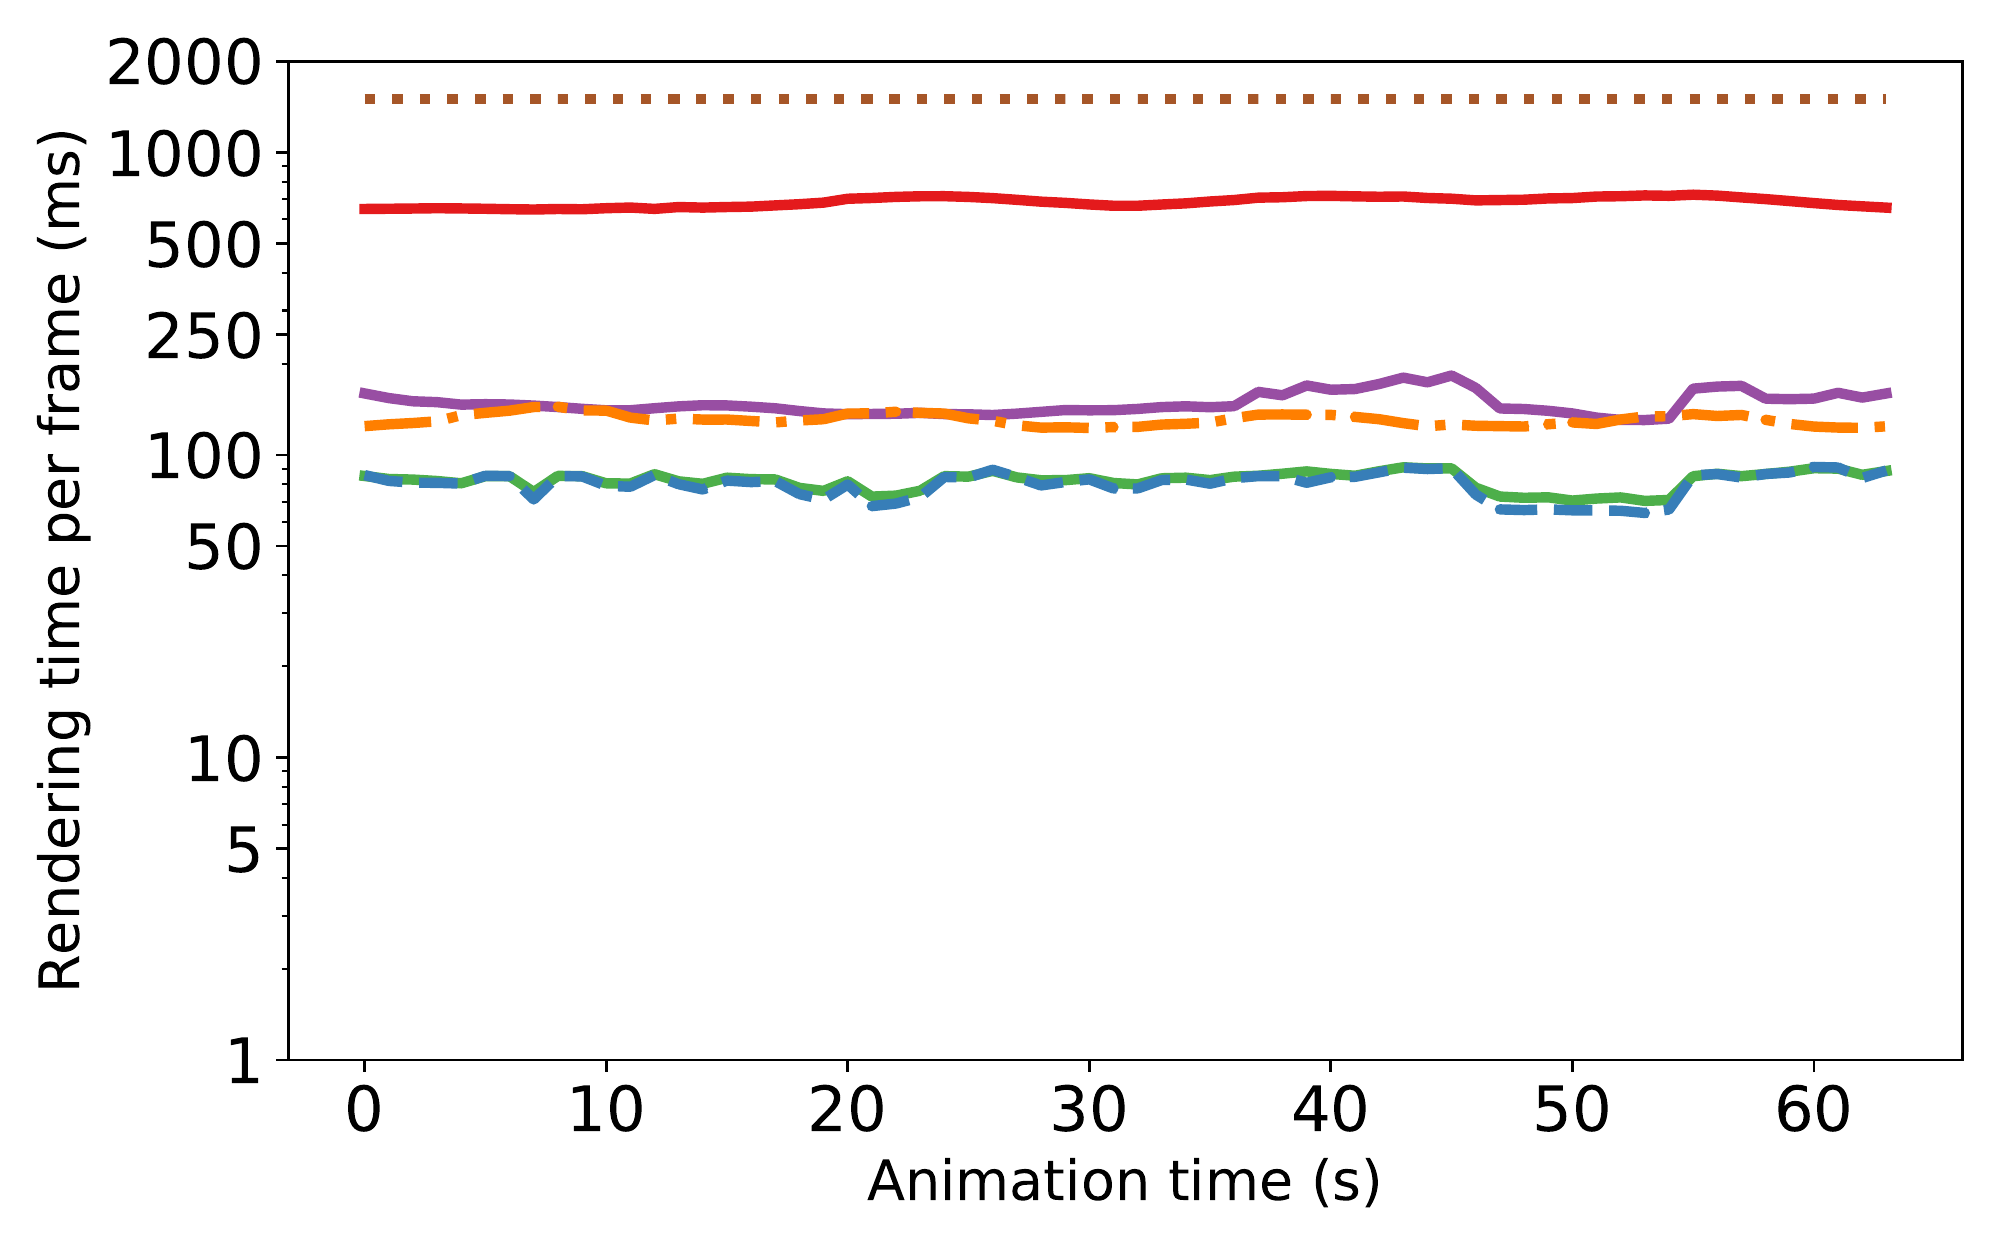}
		\put(34,15){\scriptsize\textbf{\textcolor{gray}{TURBULENCE}}}
	\end{overpic}%
	\begin{overpic}[width=0.245\textwidth,clip,trim= 00mm 0mm 2mm 2mm]
		{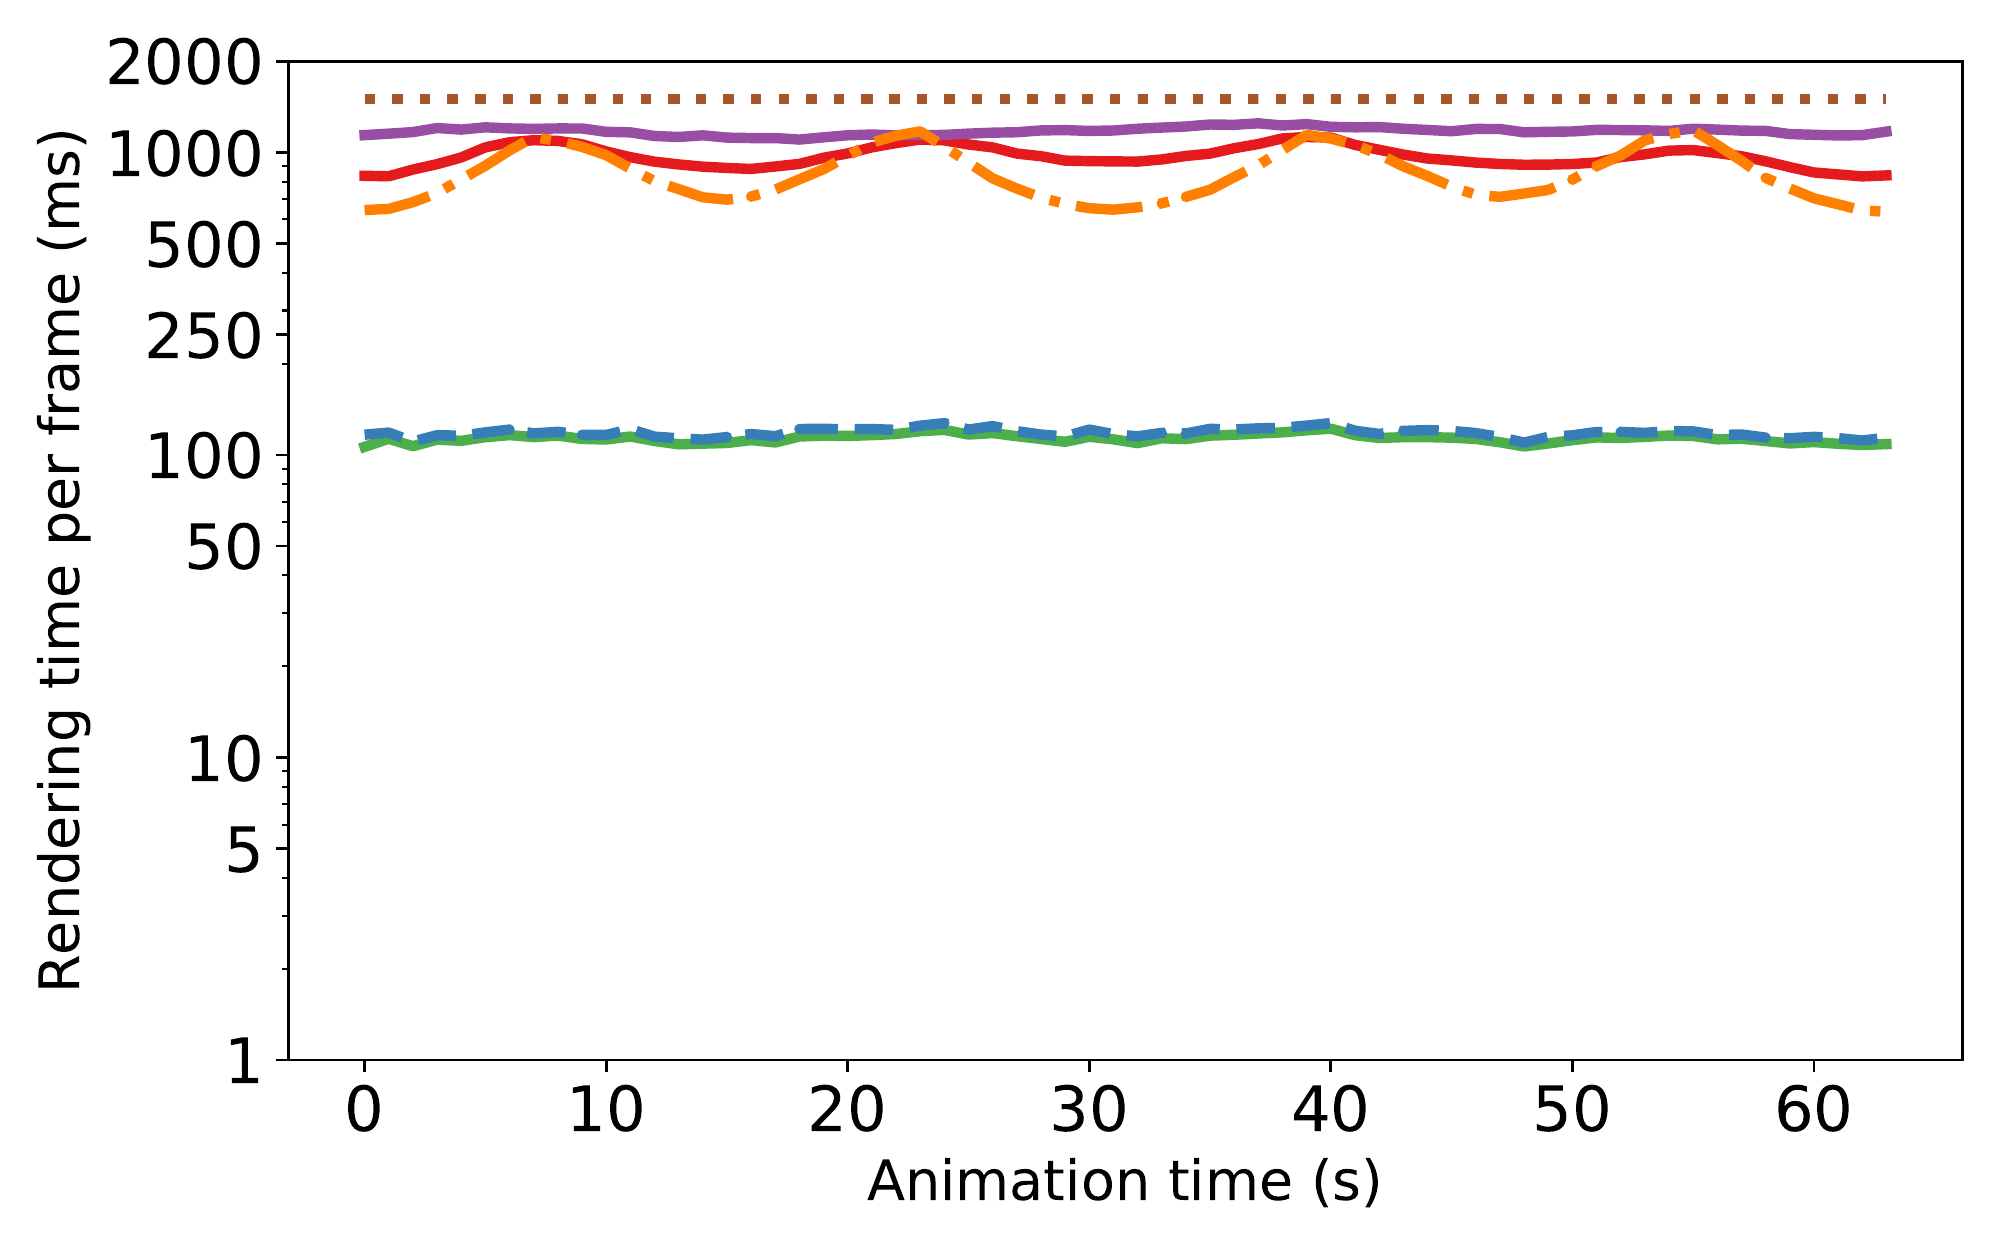}
		\put(42,15){\scriptsize\textbf{\textcolor{gray}{CLOUDS}}}
	\end{overpic}

	\caption{Rendering performance of all techniques using opaque lines (first row), transparent lines with opaque features of interest (middle), and highly transparent lines (last row). 1st, 2nd, 3rd, and 4th column are for ANEURYSM, CONVECTION, TURBULENCE, and CLOUDS respectively. For OSP, line is dotted if rendering time exceeds 1500ms.}
	\label{fig:appendix_performance}
	\vspace{15em}
\end{figure*}
\section{Rendering Performance}
\label{app:performances}
We conducted several performance tests on each data set with different transparency settings to evaluate the relation between performance and amount of transparency. Here, we rendered each data set three times along pre-recorded camera paths using different transparency settings, and we chose an appropriate zooming level for each line set to vary the amount of transparency rendering during each recorded flight.

In particular, we analyzed three different transparency settings: rendering of (a) fully opaque lines often used in visualization in terms of data exploration, (b) semi-transparent lines with features of interest rendered opaque, and (c) lines with a constant low transparency (e.g. below 0.15) to simulate extreme scenarios with many transparent layers. Note that the latter setting is used here to demonstrate how either technique behaves in this worst-case scenario, as high transparency mostly blurs out directional information. Performance measures (rendering times in milliseconds) per frame for all data sets and transparency settings are given in Fig.~\ref{fig:appendix_performance}.
